# Supplementary material for: Capping and gate control of anomalous Hall effect and hump structure in ultra-thin SrRuO$_3$ films
Source: arXiv:2007.09872 source file (2021-05-03)
Supplement: Supplementary file 1 [file Supplementary_Material.pdf]

**Supplemental Material for:**

# Capping and gate control of anomalous Hall effect and hump structure in ultra-thin $SrRuO_3$ films

Donghan Kim,[1,2] Byungmin Sohn,[1,2] Minsoo Kim,[1,2] Sungsoo Hahn,[1,2]
Youngdo Kim,[1,2] Jong Hyuk Kim,[3] Young Jai Choi,[3] and Changyoung Kim[1,2]

[1]Center for Correlated Electron Systems, Institute for Basic Science, Seoul 08826, Korea
[2]Department of Physics and Astronomy, Seoul National University, Seoul 08826, Korea
[3]Department of Physics, Yonsei University, Seoul 03722, Korea

## I. Ohmic contact for transport measurements on $SrRuO_3$/$SrTiO_3$ heterostructure films

In order to have ohmic contacts for transport measurements, we used an ultrasonic wire bonder with aluminum wires. To check whether the contact is ohmic or not, we measured the I-V character of heterostructure films. Figure S1 shows a linear I-V curve, confirming that the contact is ohmic.

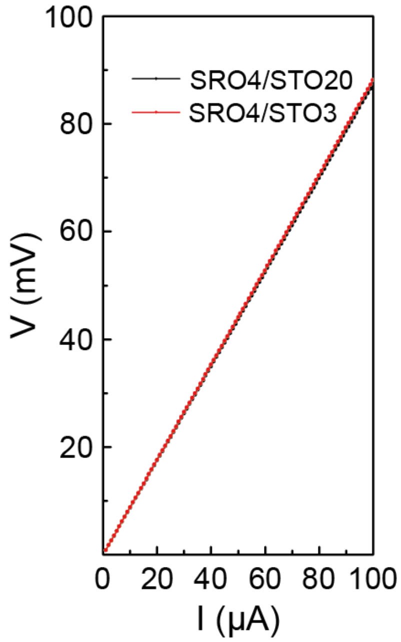


**Fig. S1.** Ohmic contact of $SrTiO_3$ (STO) capped $SrRuO_3$ (SRO) film. The I-V curve of our film shows a linear behavior, indicating an ohmic contact.

## II. Insulating properties of $SrTiO_3$ film

We measured the resistivity of a $SrTiO_3$ (STO) film on an STO substrate, which was grown under the same condition as that for the STO capping layer which is given in the main manuscript. Figure S2(a) shows a schematic of a 50 uc STO thin film on an STO (001) substrate. We measured the resistance of the STO thin film by using a 2-probe method with a multimeter as well as with a 4-probe method in a physical property measurement system (PPMS). Both of the data measured with the 2-probe and 4-probe methods showed unmeasurably high resistance. Thus, we believe that the concentration of oxygen vacancies in our STO layer is low enough not to contribute to the transport properties of the heterostructures.

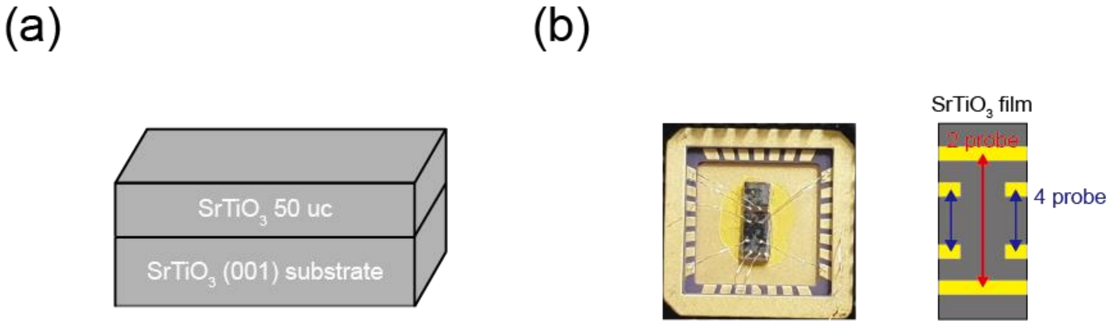


**Fig. S2.** Resistance measurements of a STO 50 uc film on a STO substrate. (a) Schematic of the measured system. (b) A photograph of the measured homoepitaxial STO film (left), and a schematic illustration of Au electrodes for resistance measurements.

## III. Effects of $SrTiO_3$ capping layer on transport properties of 4 uc $SrRuO_3$ films

We grew various thicknesses of STO capping layer on 4 unit-cell (uc) $SrRuO_3$ (SRO) films. In the data shown in Fig. S3, ferromagnetic transition temperature (Curie temperature $T_C$) is enhanced with deposition of the STO capping layer. We define $T_C$ as an anomaly in the first derivative curve, as shown in Fig. S3(b). Figure S3(c) shows Hall measurement results of STO capped 4 uc SRO thin films. Hump structure almost disappears while anomalous Hall effect (AHE) changes its sign and increases as the STO capping layer is introduced. We observed that AHEs of 10 and 20 uc STO capped 4 uc SRO films are nearly identical, suggesting that the capping layer effect is almost saturated.

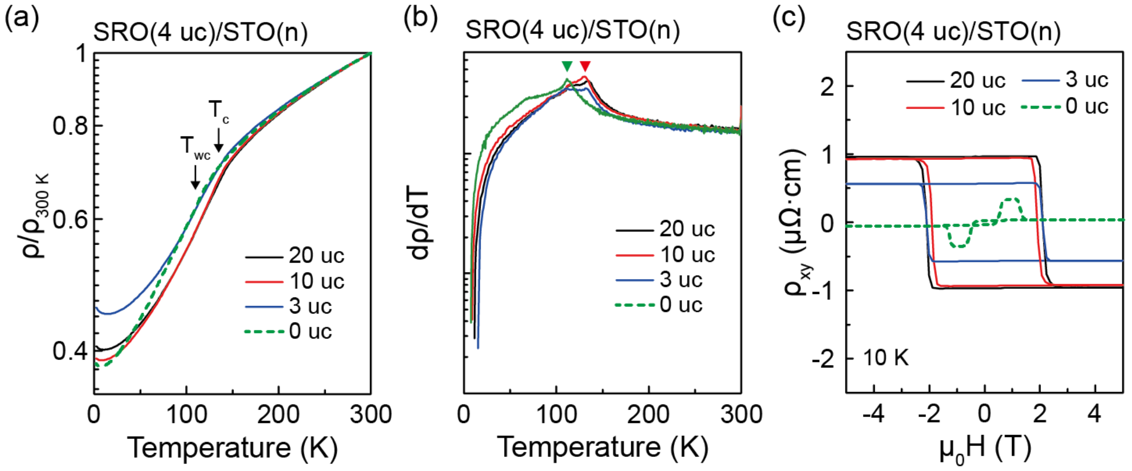


**Fig. S3.** (a) Temperature-dependent resistivity, (b) its 1st derivative, and (c) Hall resistivity of STO (*n* uc) capped SRO 4 uc films. The Curie temperature is indicated by filled inverted triangles in Fig. S3(b) which increases with deposition of the STO capping layer.

## IV. Hall effect measurements of $SrTiO_3$ capped 3 uc $SrRuO_3$ films at various temperatures

Fig. S4 below shows temperature dependent Hall measurement results, from which $\rho_{AHE}$ and $\rho_{hump}$ in Fig. 4 were extracted. $\rho_{AHE}$ and $\rho_{hump}$ are defined in the same way as described in Fig. 3(b) of the main text.

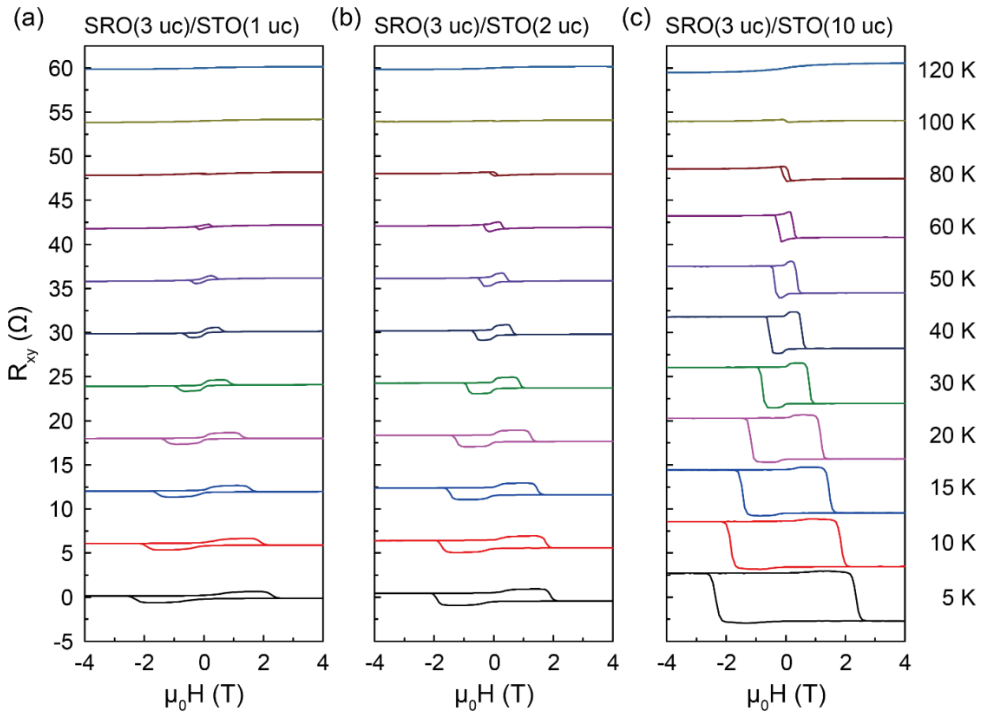


**Fig. S4.** Hall effect measurement results of (a) 1 uc, (b) 2 uc, and (c) 10 uc STO capped 3 uc SRO films at various temperatures.

## V. Incomplete disappearance of hump structure in the Hall effect

We plot $\rho_{hump}$ of 3 and 4 uc SRO films in Fig. S5(a) as a function of the STO capping layer thickness. As the thickness of the STO capping layer increases, both 3 and 4 uc SRO films show reduced $\rho_{hump}$. It appears that the hump structure disappears in the Hall effect data of STO capped 4 uc SRO films shown in Fig. 2(b) and Fig. S3(c). However, a close look of the data shows that a small hump structure remains in spite of STO capping, as seen in Fig. S5(b).

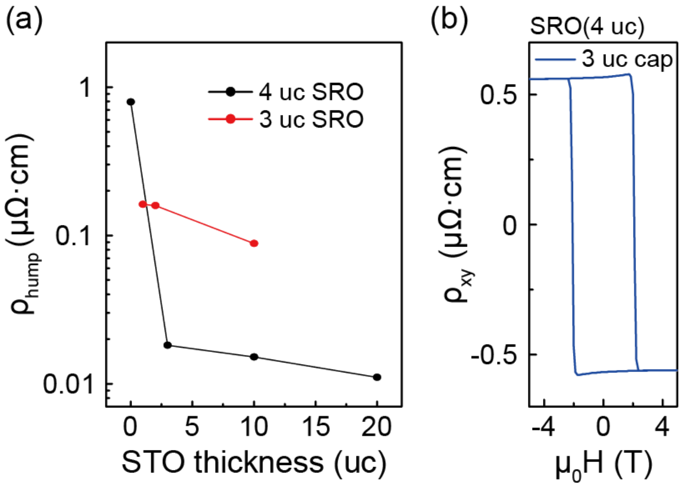


**Fig. S5.** (a) $\rho_{hump}$ plot of 3 and 4 uc SRO thin films for various STO capping layer thickness. (b) An enlarged view of the Hall measurement result of 3 uc STO capped 4 uc SRO film.
